# Supplementary material for: Online Learning of Assignments that Maximize Submodular Functions
Source: arXiv:0908.0772 source file (2009-08-05)
Supplement: Supplementary file 1 [file appendix.tex]

Lemma \ref {lem:locally_greedy} is a corollary of the following more general lemma.  The difference between the two lemmas is that, unlike Lemma \ref {lem:locally_greedy}, Lemma \ref {lem:locally_greedy_error} allows for the possibility that each $\argmax$ in the locally greedy algorithm is evaluated with additive error.  We will need this result in analyzing \OnlineGreedy later on.

%%%%%
\begin {lem} \label {lem:locally_greedy_error}
Let $f : \Feasible \to \NonNegativeReals$ be a function of the
form $f(\assignment) = f_0(\assignment) + \sum_{\k=1}^\K f_\k(\assignment \cap P_\k)$, where $f_0 :
2^\groundset \to \NonNegativeReals$ is monotone submodular, and
$f_\k : P_\k \to \NonNegativeReals$ is arbitrary for $\k \ge
1$.  Let $L = \set {\ell_1, \ell_2, \ldots, \ell_\K}$, where $\ell_\k
\in P_\k$ (for $1 \le \k \le \K$).   Suppose that for any $\k$,
\begin {equation} \label {eq:near_locally_greedy}
  f(\set {\ell_1, \ell_2, \ldots, \ell_\k})
  \ge \max_{x \in P_\k} \set { f(\set {\ell_1, \ell_2, \ldots,
  \ell_{\k-1}} + x) }  - \eps_\k \mbox { .}
\end {equation}
Then
\[
    f(L) + f_0(L) \ge \max_{\assignment \in \Feasible} \set { f(\assignment) } - \sum_{\k=1}^\K \eps_\k \mbox { .}
\]
\end {lem}
\begin {proof}
Let $\OPT = \argmax_{\assignment \in \Feasible} \set { f(\assignment) }$, and let $\OPT = \set
{o_1, o_2, \ldots, o_\K}$, where $o_\k \in P_\k$ (for $1 \le \k \le \K$).  Define
\[
    \Delta_\k(L) := f_\k(\set{o_\k}) + f_0(L \cup \set { o_1, o_2,
    \ldots, o_\k })
- f_0(L \cup \set { o_1, o_2, \ldots, o_{\k-1} }) \mbox { .}
\]
Let $L_\k = \set {\ell_1, \ell_2, \ldots, \ell_{\k-1}}$.
Using submodularity of $f_0$, we have
\begin {align*}
\Delta_\k(L) & \le  f_\k(\set{o_\k}) + f_0(L_\k + o_\k) - f_0(L_\k) \\
    & = f(L_\k + o_\k) - f(L_\k) \\
    & \le f(L_\k + \ell_\k) - f(L_\k) + \eps_\k  \mbox { .}
\end {align*}
Then, using monotonicity of $f_0$,
\begin {align*}
f(\OPT)
    & \le f_0(L \cup \OPT) + \sum_{\k=1}^\K f_\k(\OPT \cap P_\k) \\
    & = f_0(L) + \sum_{\k=1}^\K \Delta_\k(L) \\
    & \le f_0(L) + \sum_{\k=1}^\K f(L_\k + \ell_\k) - f(L_\k) + \eps_\k \\
    & = f_0(L) + f(L) - f(\emptyset) + \sum_{\k=1}^\K \eps_\k \mbox { .}
\end {align*}
Rearranging this inequality and using $f(\emptyset) \ge 0$ completes the proof.
\end {proof}
%%%%%

To analyze \OnlineGreedy, we will also need Theorem \ref {thm:offline_greedy_error}, which is a generalization of Theorem \ref {thm:offline_greedy}.

%%%%%
\begin {thm} \label {thm:offline_greedy_error}
Suppose $f$ is monotone submodular.
Let $G = \set {g_{\k,\j}: \k \in \bracket{\K}, \j \in \bracket {\J} }$,
where $g_{\k,\j} \in \P_\k$ for all $\k$ and $\j$.
Suppose that for all $\k \in \bracket{\K}$ and $\j \in \bracket{\J}$,
\begin {equation} \label {eq:epsilon}
  F(G^-_{\k,\j} + g_{\k,\j}) \ge
  \max_{x \in \P_\k \times \set{\j}} \set { G^-_{\k,\j} + x  } - \eps_{\k,\j}
\end {equation}
where $G^-_{\k,\j} = \set { g_{\k', \j'}: \k' \in \bracket{\NumPartitions}, \j' < \j } \cup \set {
g_{\k',\j}: \k' < \k }$ (i.e., $G^-_{\k,\j}$ equals $G$ just
before $g_{\k,\j}$ is added).
Then
$  f(G) \ge \beta(\J, \K) \cdot \max_{\assignment \in \Feasible} \set {f(\assignment)} -
  \sum_{\k=1}^\K \sum_{\j=1}^\J \eps_{\k,\j}$,
where $\beta(\J, \K)$ is defined as $1 - (1 - \frac {1} {\J})^\J - {\K \choose 2} \J^{-1} $.
\end {thm}
\begin {proof}
The proof is identical to the proof of Theorem \ref {thm:offline_greedy} in the main text, using Lemma \ref {lem:locally_greedy_error} in place of Lemma \ref {lem:locally_greedy}.
\end {proof}
%%%%%

Finally, we prove Theorem \ref {thm:online_greedy}, which we restate here for convenience.
%%%%%
\newtheorem{thmonlinegreedy}{Theorem \ref{thm:online_greedy}}
\begin {thmonlinegreedy}
Let $\Regret_{\k,\j}$ be the regret of $\Alg_{\k,\j}$, and let $\beta(\K,
\J) = 1 - \paren { 1 - \frac 1 \J }^\J - {\K \choose 2} \J^{-1}$.
Then
\[
    \E { \sum_{t=1}^T f_t(G_t) } \ge \beta(\K, \J) \cdot \max_{\assignment \in \Feasible} \set { \sum_{t=1}^T f_t(\assignment) } - \E { \sum_{\k=1}^\K \sum_{\j=1}^\J \Regret_{\k,\j} } \mbox { .}
\]
\end {thmonlinegreedy}
\begin {proof}
The idea of the proof is to view \OnlineGreedy as a version of
\OfflineGreedy that, instead of greedily selecting single (element,color) pairs
$g_{\k,\j} \in \P_\k \times
\set {\j}$, greedily selects (element vector, color) pairs
$\vec g_{\k,\j} \in \P_\k^T \times \set {\j}$, where $T$ is the number of rounds.

First note that for any $\k \in \bracket{\K}$, $\j \in \bracket {\J}$,
and $x \in \P_\k \times \set{\j}$,
by definition of $\Regret_{\k,\j}$ we have
\[
  \sum_{t=1}^T \bar F_t\paren{G^t_{\k,\j} + g^t_{\k,\j}} \ge
  \paren{\sum_{t=1}^T \bar F_t\paren{G^t_{\k,\j} + x}} -\Regret_{\k,\j} \mbox { .}
\]
Taking the expectation of both sides over $\Color$, and choosing $x$
to maximize the right hand side, we get
\begin {equation} \label {eq:expected_regret}
  \sum_{t=1}^T F_t\paren{G^t_{\k,\j} + g^t_{\k,\j}} \ge
  \max_{x \in \P_\k \times \set{\j}} \set { \sum_{t=1}^T F_t\paren{G^t_{\k,\j} + x} } - \eps_{\k,\j}
\end {equation}
where we define $F_t(\assignment) = \Esub{\cvec}{f_t(\sample_{\cvec}(\assignment))}$ and
$\eps_{\k,\j} = \E {\Regret_{\k,\j}}$.

We now define some additional notation.
For any set $\vec S$ of vectors in $\groundset^T$, define
\[
  f(\vec S) = \sum_{t=1}^T f_t\paren{\set{\vec a_t: \vec a \in \vec
  S}} \mbox { .}
\]
Next, for any set $\vec S$ of (element vector, color) pairs in
$\bigcup_{\k=1}^\K (\P_\k^T
\times \set {\j})$, define $\sample_{\cvec}(\vec S) = \bigcup_{\k=1}^\K
\set { \vec x \in \P_\k^T: (\vec x, \Color_\k) \in \vec S  }$.
Define $F(\vec S) = \Esub{\cvec}{f(\sample_{\cvec}(\vec S))}$.
By linearity of expectation,
\begin {equation} \label {eq:linexp}
  F(\vec S) = \sum_{t=1}^T F_t\paren{\set { (\vec x_t, \j): (\vec x, \j)
  \in \vec S  }} \mbox { .}
\end {equation}
Let $\vec g_{\k,\j} = (\vec x, \j)$, where $\vec x$ is such that $(\vec
x_t, \j) = g^t_{\k,\j}$ for all $t \in \bracket{T}$.
%Let $\vec g_{\k,\j} = (\tuple{g_{\k,\j}^1, g_{\k,\j}^2, \ldots, g_{\k,\j}^T} , \j)$.
Analogously to $G^{t-}_{\k,\j}$, define
$\vec G^-_{\k,\j} = \set {\vec g_{\k',
\j'}: \k' \in \bracket{\K}, \j' < \j} \cup \set {\vec g_{\k',\j}: \k' < \k }$.
By \eqref {eq:linexp}, for any $(\vec x, \j) \in \groundset^T \times \bracket{\J}$ we have
$F(\vec G^-_{\k,\j} + (\vec x, \j)) = \sum_{t=1}^T F_t(G^{t-}_{\k,\j} +
(\vec x_t, \j))$.
Combining this with \eqref {eq:expected_regret}, we get
\begin {equation} \label {eq:goal}
  F\paren{\vec G^-_{\k,\j} + \vec g_{\k,\j}} \ge \max_{a: a \in \P_\k} \set {
  F\paren{\vec G^-_{\k,\j} + (a^T, \j)} } - \eps_{\k,\j}
\end {equation}
where $a^T$ is the unique element of $\set{a}^T$.
Having proved \eqref {eq:goal}, we can now use Theorem \ref
{thm:offline_greedy_error} to complete the proof.
Let $\vec P_\k := \set {a^T: a \in P_\k}$ for each $\k \in \bracket{\K}$,
and define a new partition matroid over ground set $\set{a^T : a \in \groundset}$
with feasible solutions
$\vec \Feasible := \set{ \vec \assignment : \forall
\k \in \bracket{\K}, |\vec \assignment \cap \vec \Partition_\k| \le 1}$.
%Let $\vec P = \set{\vec P_1, \vec P_2, \ldots, \vec P_\K}$ define a new
%simple partition matroid over ground set $\set{a^T :
%a \in \groundset}$, where $\vec P_\k = \set {a^T: a \in P_\k}$, and
Let $\vec G = \set {\vec g_{\k,\j}: \k \in \bracket{\K}, \j \in \bracket{\J}}$.
As argued in the proof of Lemma \ref {lem:outer_loop},
$F_t$ is monotone submodular.  Using this fact together with \eqref
{eq:linexp}, it is straightforward to show that $F$ itself is monotone
submodular.  Thus by Theorem \ref {thm:offline_greedy_error},
\[
  F(\vec G) \ge \beta(\J,\K) \cdot \max_{\vec \assignment \in \vec \Feasible} \set {
  f(\vec \assignment) } - \sum_{\k=1}^\K \sum_{\j=1}^\J \eps_{\k,\j} \mbox { .}
\]
To complete the proof, it suffices to show that
$F(\vec G) = \E {\sum_{t=1}^T f_t(G_t) }$, and that
$\max_{\vec \assignment \in \vec \Feasible} \set {f(\vec \assignment)} \ge \max_{\assignment \in \Feasible}
\set { \sum_{t=1}^T f_t(\assignment) }$.  Both facts follow easily from
the definitions.
\end {proof}
%%%%%
